# Supplementary material for: A Controllable Model of Grounded Response Generation
Source: arXiv:2005.00613 source file (2021-06-14)
Supplement: Supplementary file 1 [file appendix.tex]

\appendix
\section{Control Phrase Prediction Assessment}
\label{sec:appendix}

As an intermediate assessment of the content planner, we report the Precision, Recall and F1 of tokens in \CnN and \GrCnN, with respect to reference responses (counts for stop-words and punctuation tokens are removed) in Table~\ref{intermediate}. For each test dialogue context, we calculate the values for the reference response that gives the highest F1 score and report the average among all test examples for each metric. We notice that the retrieved-based content planner predicts slightly better quality phrases than BERT QA, while still worse than the gold control phrases from the carved out human response. A possible reason that BertQA performs worse in defining gold control phrases could be that, during training, the supervised answers for each query (dialogue context) and document (grounding) given to the model include all string spans that match each gold control phrase, which potentially contain noise.

\begin{table}[h]%
\centering
\begin{adjustbox}{width=0.48\textwidth}
\begin{tabular}{@{\hskip3pt}l@{\hskip3pt}|@{\hskip3pt}l@{\hskip5pt}l@{\hskip5pt}l@{\hskip5pt}|l@{\hskip5pt}l@{\hskip5pt}l@{\hskip5pt}}
\hline \textbf{Content Planner} & \textbf{C-P} & \textbf{C-R} &  \textbf{C-F}  & \textbf{G-P} & \textbf{G-R}  & \textbf{G-F} \\ \hline
Retrieval-based  & 13.8\% & 5.6\% & 7.2\% & 5.5\% & 21.8\% & 7.7\% \\
BertQA & 14.7\% & 4.8\% & 6.5\% & 5.0\% & 21.3\% & 7.1\% \\ \hline
Human & 24.4\% & 6.1\% & 8.6\% & 6.6\% & 17.2\% & 8.0\% \\
\hline
\end{tabular}
\end{adjustbox}
\caption{\label{intermediate} Response coverage of control phrase \CnN and associated grounding \GrCnN tokens.}
\end{table}

Table~\ref{more-examples} shows more example outputs from systems in our experiment.

\begin{table*}
\small
\centering
\begin{adjustbox}{width=1.0\textwidth}
\begin{tabular}{p{1.6cm}|p{11cm}}
\hline 
Dialogue Context & More cops have died of illness linked to 9/11 than had perished in it on that day.\\
Control &  \textbf{people died}; \textbf{elevators}\\
Grounding & ... 1,402 \textbf{people died} at or above the floors of impact in the north \textbf{tower}. ... many \textbf{elevators} did not plunge, but were destroyed due to the crash and subsequent fires, or were stranded in the shafts. ...\\
\hline
\Xt & I'm not sure if this is true, but I'm pretty sure it's true.\\
\Xt{}\Cn & I'm pretty sure the \textbf{elevators} were not meant to be elevated above the \textbf{elevators}.\\
\Xt{}\Cn{}\GrCn &  I'm surprised that the number of \textbf{people died} in the \textbf{elevators} is low.\\
\Xt{}\Cn{}\GrCn+IA & I'm pretty sure the number of \textbf{people died} in the \textbf{elevators} is higher than the number of \textbf{people died} in the \textbf{towers}.\\
\Xt{}\CnN{}\GrCnN+IA & I'm pretty sure the 9/11 attacks were the most horrific of the world trade center attacks.\\

\hline \hline
Dialogue Context & In 1997 a killer whale held a great white shark upside down for 15 minutes, causing it to suffocate, after which it ate only its liver \\
Control &  \textbf{orca} \\
Grounding & ... The \textbf{orca} held the \textbf{shark} upside down to induce tonic immobility and kept the \textbf{shark} still for fifteen minutes , causing it to suffocate ... The \textbf{orca} then proceeded to eat the dead shark 's liver ...\\
\hline
\Xt &  I think the article is about a great white \textbf{shark}.\\
\Xt{}\Cn & I'm not sure if this is the \textbf{orca} that killed the killer whale, but i think it's the killer whale that killed the killer whale.\\
\Xt{}\Cn{}\GrCn &  I think the \textbf{orca} is the one who's the bad guy.\\
\Xt{}\Cn{}\GrCn+IA &  I'm pretty sure the \textbf{orca} is the one who killed the \textbf{shark}.\\
\Xt{}\CnN{}\GrCnN+IA &  I'm pretty sure that's a great white \textbf{shark}.\\

\hline \hline
Dialogue Context & Millions of Puerto Ricans just lost power again after a line repaired by Whitefish Energy failed.\\
Control &  \textbf{restored}\\
Grounding & ... just 18\% of the territory now has \textbf{power}, and officials did not have a clear timeline on when the \textbf{power} will be \textbf{restored}. ...\\
\hline
\Xt & I'm not sure if this is true, but I'm pretty sure it's true.\\
\Xt{}\Cn & I'm not surprised. I'm surprised that the government is still trying to get the rest of the population \textbf{restored}.\\
\Xt{}\Cn{}\GrCn & I'm surprised they didn't just repair the line. I mean, it's not like they were going to be able to get back to the island they were supposed to be.  \\
\Xt{}\Cn{}\GrCn+IA & I'm surprised they didn't just \textbf{restore power}.\\
\Xt{}\CnN{}\GrCnN+IA & I'm from San Juan and I'm pretty sure I'm not the only one that noticed this.\\

\hline
\end{tabular}
\end{adjustbox}
\caption{\label{more-examples} More sample outputs of the systems, with baseline outputs for comparison.}
\end{table*}
